# Supplementary material for: Deep Learning with Tabular Data: A Self-supervised Approach
Source: arXiv:2401.15238 source file (2024-01-26)
Supplement: Supplementary file 1 [file AppendixTemplate.tex]

% Appendix Template

\chapter{Appendix Title Here} % Main appendix title

\label{AppendixX} % Change X to a consecutive letter; for referencing this appendix elsewhere, use \ref{AppendixX}

Write your Appendix content here.
